# Supplementary material for: Kondo-lattice ferromagnets and their peculiar order along the magnetically hard axis
Source: arXiv:1901.04288 ancillary file (2019-03-18)
Supplement: Supplementary file 1 [file KLF_SMI.pdf]

**Supplementary Information for**  
**Kondo-lattice ferromagnets and their peculiar order**  
**along the magnetically hard axis**

D. Hafner,<sup>1</sup> Binod K. Rai,<sup>2</sup> J. Banda,<sup>1</sup> K. Kliemt,<sup>3</sup> C. Krellner,<sup>3</sup>  
J. Sichelschmidt,<sup>1</sup> E. Morosan,<sup>2</sup> C. Geibel,<sup>1</sup> and M. Brando<sup>1</sup>

<sup>1</sup>*Max Planck Institute for Chemical Physics of Solids, D-01187 Dresden, Germany*

<sup>2</sup>*Department of Physics and Astronomy, Rice University, Houston, Texas 77005, USA*

<sup>3</sup>*Physikalisches Institut, Johann Wolfgang Goethe-Universität, D-60438 Frankfurt am Main, Germany*

# CONTRADICTION BETWEEN EXCHANGE INTERACTIONS DETERMINED FROM INELASTIC NEUTRON SCATTERING AND SUSCEPTIBILITY AT HIGH TEMPERATURES.

A direct approach to get information on the exchange interaction is to measure the dispersion relation of magnetic excitations, e.g. magnons, using inelastic neutron scattering (INS). Therefore one might expect that the anisotropy of the exchange interactions in the ferromagnetic (FM) systems discussed in the main part of our paper is a problem which can unambiguously be settled using this approach. For one of the compounds discussed in our paper, CeAgSb<sub>2</sub>, such a detailed INS study has been performed [37]. This study indeed concludes that all the experimental results, including the FM ordering along the hard  $c$ -axis, can be fully explained by a huge anisotropy of the exchange interactions. However, we shall argue in the following that, in contrast to the view suggested in [37], the magnon dispersion relations typically determined by INS do not provide on their own a unique answer to the values of the exchange interactions. Specifically in the case of CeAgSb<sub>2</sub>, we shall demonstrate that the huge anisotropy of the exchange parameters deduced from INS in [37] are in clear contradiction to the anisotropy of the susceptibility observed at high temperatures. This contradiction points on its own to a yet unidentified phenomena which promotes the hard axis ordering at low temperature. Further on, we show that a similar discrepancy between a huge anisotropy of exchange interactions deduced from INS results [55] and a much weaker anisotropy of the susceptibility at high temperature is also observed in the system CeRu<sub>2</sub>Al<sub>10</sub> with antiferromagnetic (AFM) order along the hard axis. Thus, the problem addressed in our paper is not only relevant to FM, but also to AFM Kondo systems.

The detailed study performed in [37] on CeAgSb<sub>2</sub> provides a very good basis to illustrate the problem. CeAgSb<sub>2</sub> is a well-studied tetragonal Kondo-lattice system which orders ferromagnetically at  $T_C = 9.5$  K with moment along the  $c$ -axis, despite the  $ab$  in-plane moment of the crystalline electric field (CEF) ground state doublet being more than a factor of 3 larger than the out of plane moment. S. Araki *et al.* determined the magnon dispersion relation in the FM phase using INS, fitted these data with a model including ten different exchange parameters, and concluded that all the properties observed in this compound could be well reproduced by this model [37]. In particular the ordering with moment along the hard CEF axis was attributed to a huge anisotropy of the ( $\mathbf{k} = 0$ ) mean field exchange parameters  $\lambda$ , with  $\lambda_z = 167$  mol/emu for the  $c$ -axis component of the moment being one order of magnitude larger than  $\lambda_\perp = 14$  mol/emu for the in-plane component of the moment [37].

The essence of the problem in the analysis of the INS data is that these data were obtained deep into the FM phase at  $B = 0$  and  $T \ll T_C$ . Under these conditions the moment is fully polarized along the ordering direction (for clarity we shall call this direction the  $z$  direction, in accordance with [37]), and therefore the dispersion is essentially only sensitive to the exchange components transversal to the ordered moment. That is for instance clearly seen in the relation which determines the dispersion relation, see e.g. equation (8) and (9) in [37]:

$$\omega_{\mathbf{k}} = \Delta + \frac{9}{2}[I_\perp(\mathbf{0}) - I_\perp(\mathbf{k})] \quad (8)$$

$$\Delta = \frac{1}{2}[I_z(\mathbf{0}) - 9I_\perp(\mathbf{0})]. \quad (9)$$

In these equations all the Fourier components of the transverse exchange,  $I_\perp(\mathbf{0})$  and  $I_\perp(\mathbf{k})$  enter, but only the  $\mathbf{k} = 0$  component of the longitudinal exchange  $I_z(\mathbf{0})$  is relevant. Accordingly, in the Table III of [37] which lists the exchange interactions determined from the neutron data, 9 different interaction parameters as well as  $I_z(\mathbf{0})$  are listed for the transverse direction, while for the  $z$  direction only one parameter,  $I_z(\mathbf{0})$ , is given. At first glance, equations (8) and (9) suggest that the neutron data allow for an independent determination of  $I_z(\mathbf{0})$ . This is also suggested in [37], where it is stated “The  $I_\perp^n$  obtained by fitting dispersion [...] are listed in Table III”. However that is not true. As one can easily see from equations (8) and (9), the neutron data only determine  $I_z(\mathbf{0})$ ,  $I_\perp(\mathbf{0})$  and  $I_\perp(\mathbf{k})$  up to an arbitrary constant. If a given set of  $I_z(\mathbf{0})$ ,  $I_\perp(\mathbf{0})$  and  $I_\perp(\mathbf{k})$  fit the experimental data, than any set where  $I_z(\mathbf{0})$  was increased by a fixed value  $A$ ,  $I_z^*(\mathbf{0}) = I_z(\mathbf{0}) + A$ , and  $I_\perp(\mathbf{0})$  and  $I_\perp(\mathbf{k})$  were increased by  $A/9$ ,  $I_\perp^*(\mathbf{0}) = I_\perp(\mathbf{0}) + A/9$  and  $I_\perp^*(\mathbf{k}) = I_\perp(\mathbf{k}) + A/9$ , shall fit the data as well. Therefore the neutron data on their own do not allow for an independent determination of all parameters  $I_z(\mathbf{0})$ ,  $I_\perp(\mathbf{0})$  and  $I_\perp(\mathbf{k})$ . Instead, in order to determine these parameters, one of the parameters  $I_z(\mathbf{0})$  or  $I_\perp(\mathbf{0})$  has to be fixed from a different experiment. The usual way, and that is also the way which we suspect was used in [37], is to fix  $I_z(\mathbf{0})$  using the ordering temperature  $T_C$ . In the simple mean field approximation  $T_C = \lambda_z C_z^{LT}$  where  $\lambda_z$  is the exchange constant for the  $c$  direction, which is proportional to  $I_z(\mathbf{0})$ , and  $C_z^{LT}$  is the Curie constant for the  $c$  direction at low  $T$ . In the case of CeAgSb<sub>2</sub> the CEF ground state (being a  $\Gamma_6$  state) leads to an effective  $J = 1/2$  for the  $c$  direction, and thus to  $C_z^{LT} = (g_J \mu_B)^2 J(J+1)/(3k_B) = 0.0689$  K·emu/mol. With the experimental  $T_C = 9.5$  K this most simple approach results in  $\lambda_z = 138$  mol/emu, close to the value proposed

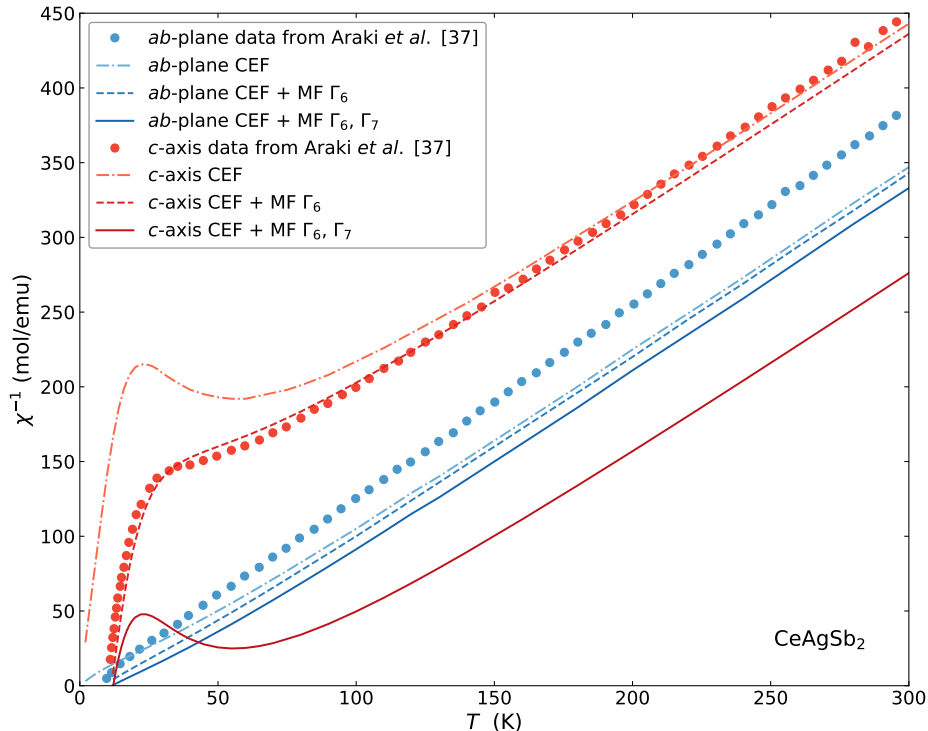

FIG. S1. T-dependence of the in-plane (blue) and out of plane (red) inverse susceptibility of  $\text{CeAgSb}_2$ . The dots correspond to the measured susceptibilities published in [37]. The dash-dotted lines correspond to the susceptibilities expected from the CEF scheme of  $\text{CeAgSb}_2$  in the absence of exchange interactions. We used the same CEF parameters as [37] and thus these curves are identical to the corresponding ones in [37]. The dashed line is obtained when adding to the CEF a mean field exchange acting only on the CEF  $\Gamma_6$  ground state doublet, as done in [37]. Here, our results are identical to those in [37], too. The out of plane inverse susceptibility  $\chi_c^{-1}$  seems to reproduce the experimental results nicely. However, when including the effect of the same exchange on the excited CEF doublets, the resulting curve for the out of plane curve (red solid line) strongly deviates from the experimental result leading to an inversion of the anisotropy at high temperatures. This points to a severe problem associated with exchange parameters deduced from the standard mean field analysis of INS data. For  $\chi_{ab}^{-1}$ , the difference between the three calculated results is quite small because the exchange parameter proposed by [37] is tiny in this direction.

in [37],  $\lambda_z = 167 \text{ mol/emu}$ . Thus, in this kind of studies the determination of all exchange interactions rely on the assumption that the ordering temperature is correctly given by the mean field approach, implicitly assuming the absence of any further effects affecting  $T_C$  or  $T_N$ . Therefore the claim in [37], as well as in a number of similar studies, that the ordering along the hard direction is due to a huge anisotropy of the exchange interaction, completely relies on the assumption that the ordering temperature is entirely determined by mean field and that there is no further effect. Thus, to some extent this is a circular argument.

As evident from the above analysis, assuming  $T_C$  to be fully determined by mean field,  $T_C = 9.5 \text{ K}$  and ordering along the hard direction necessarily implies a large  $\lambda_z$  of the order of  $140 \text{ mol/emu}$  in  $\text{CeAgSb}_2$ . However, this results in a strong incompatibility when reproducing the experimental susceptibility at high T, a problem which was not recognized in [37]. In [37] the authors also calculated the temperature dependence of the susceptibility along the  $c$  direction and the basal plane up to  $T = 300 \text{ K}$  using a Hamiltonian which includes the CEF, the effect of an external field, and an anisotropic mean field exchange, and compared the results of their calculation with experimental data in Fig. 12, which we reproduced in Fig. S1. They claimed an excellent agreement, and indeed for the  $c$  direction the agreement is very good, while for the in-plane direction there is a deviation at higher temperature, which however is likely due to a problem in the experimental data. But a closer look to Fig. S1 reveals a severe problem, which is neither mentioned nor discussed in [37]. At low temperatures  $T < 20 \text{ K}$ , the  $\chi_c^{-1}(T)$  curve (red dashed line) calculated for CEF + exchange is significantly shifted downwards compared to the calculation for only CEF (red dash-dotted line), in perfect agreement with the huge FM exchange. Indeed at  $T \approx 10 \text{ K}$  the vertical shift amounts

to about -160 mol/emu, as expected from  $\lambda_z = 167$  mol/emu. However, with increasing temperature this shift rapidly decreases and almost vanishes for  $T > 150$  K. That would imply that the exchange interactions decrease rapidly with increasing temperature and almost vanish above 150 K. This is very unlikely to be the case. This strange behavior in the calculated CEF + exchange curve has its origin in the Hamiltonian that the authors used to calculate the susceptibility at high temperature, (equation (10) in [37]). In this exchange term,  $H_{\text{exch}} = gJ\mu_B \sum_{\alpha} h^{\alpha} J_{\Gamma_6}^{\alpha}$ , solely the contribution of the  $\Gamma_6$  CEF ground state is considered, while the contributions of the excited CEF levels are entirely omitted. That might be appropriate at low temperature, the temperature range to which most of the paper is dedicated, but is certainly inappropriate for  $T > 25$  K, where the excited CEF levels come into play. Including the effect of exchange on the excited CEF levels shifts the  $\chi_c^{-1}(T)$  curve downwards by 167 emu/mol not only at low, but at any temperature. We add this curve in Fig. S1 (red solid line). The resulting CEF + exchange  $\chi_c^{-1}(T)$  curve is far below the experimental results for  $T > 50$  K, it even crosses the  $\chi_{ab}^{-1}(T)$  curve for in-plane field, resulting in an inversed anisotropy of the susceptibility for  $T > 150$  K. Thus  $\lambda_z = 167$  mol/emu proposed by [37] leads to a complete disagreement between calculated and experimental susceptibility at high temperature when including exchange on excited CEF levels.

This argument can be put on a more general basis. It has long been shown that exchange interaction and CEF effects are just additive in determining the anisotropic Curie-Weiss temperature, see e.g. Ref. [S1]. Concerning the effect of CEF, the anisotropic Curie-Weiss temperatures  $\theta_{ab}$  and  $\theta_c$  only depend on the second order CEF parameter  $B_2^0$ . For Ce,  $\theta_{ab} - \theta_c = 9.6B_2^0$ , see e.g. equation (3) in [S2]. The CEF of CeAgSb<sub>2</sub> has been the subject of many studies, and all these studies yield a similar CEF scheme. Therefore, the possible range for  $B_2^0$  is quite limited,  $B_2^0 = 7.1 \pm 0.7$  K. This implies that  $\theta_{ab} - \theta_c \approx 68$  K. Instead of using the Curie Weiss temperatures, which require an extrapolation of the  $\chi^{-1}(T)$  plots from high to low temperatures, it is more convenient to use the corresponding vertical shift of the  $\chi^{-1}(T)$  curves. In analogy to the exchange interaction we shall call this shift  $\lambda_{CEF}$ , with  $\lambda_{CEF} = (\theta_{ab} - \theta_c)/C$  were  $C$  is the usual high temperature Curie constant,  $C = 0.802$  mol/emu for Ce. Therefor for CeAgSb<sub>2</sub>  $\lambda_{CEF} = 85$  mol/emu. Thus at high temperatures  $T > 150$  K, the CEF alone is expected to shift the  $\chi_c^{-1}(T)$  curve by 85 mol/emu above the  $\chi_{ab}^{-1}(T)$  curve. According to Fig. 12 in [37], the total shift  $\lambda_t$  between the experimental  $\chi_{ab}^{-1}(T)$  and  $\chi_c^{-1}(T)$  curves at high temperature is about 65 mol/emu. However the difference in the slope of the experimental  $\chi_{ab}^{-1}(T)$  curve and the calculated one indicate some problems in the experimental data, which would result in an underestimation of  $\lambda_t$ . Indeed the results in Fig. 9 of [39], where the slope of the  $\chi^{-1}(T)$  plots at high temperature agrees for both directions very well with the expectation, indicates a slightly larger  $\lambda_t = 82$  mol/emu. But both results show that the observed anisotropy in  $\chi^{-1}(T)$  at high temperature is to a large extent, at least 80%, accounted for by the effect of the CEF. This implies that the anisotropy in the mean field exchange parameter  $\lambda$  at high temperatures cannot be large, at most of the order of 20 mol/emu, one order of magnitude less than the anisotropy proposed by [37].

Comparing the measured susceptibilities with those calculated on the basis of the CEF model results in a further contradiction with the exchange parameter deduced from the INS data in [37]. In such local moment systems the differences between the measured susceptibilities and those calculated with a reliable CEF model can be attributed to the exchange interactions. At high temperatures the only relevant CEF parameter is  $B_2^0$ . As stated above, for CeAgSb<sub>2</sub> this parameter is known quite precisely from other properties. Therefore at high temperatures the CEF based susceptibilities of CeAgSb<sub>2</sub> can be predicted with high reliability. As evident from Fig. S1, at high temperatures the measured inverse in-plane susceptibility is systematically and significantly above the CEF one. This implies that the mean field exchange parameter for the xy-component of the moment is negative with  $\lambda_{\perp} \approx -34$  mol/emu. Thus this exchange is dominated by sizeable AFM interactions. For the  $c$  direction experimental and CEF calculations are close together at high temperature, implying that ( $\mathbf{k} = 0$ ) mean field exchange parameter  $\lambda_z$  is very small. Taking other published experimental susceptibility data [34, 39] lead to essentially the same result with  $-38 \text{ mol/emu} < \lambda_{\perp} < -30 \text{ mol/emu}$  and  $-20 \text{ mol/emu} < \lambda_z < +2 \text{ mol/emu}$ . Thus comparing the measured susceptibilities of CeAgSb<sub>2</sub> with those calculated from the well-established CEF model unequivocally implies dominant and sizeable AFM exchange for the in-plane-component of the moment and a weak mean field exchange parameter for the  $z$  component of the moment. This is in complete contradiction to the conclusion of [37] based on the analysis of the INS measurements, which claimed a huge FM interaction for the  $c$ -component and a much weaker and predominantly FM exchange for the in-plane component. On the other hand, the observed FM ordering with moment along the hard CEF  $c$  direction is within a mean field approach incompatible with the exchange parameters deduced from the high temperature susceptibility. The huge discrepancy between the exchange parameters required within a mean field approach to account for the hard axis FM ordering at low temperature, and the exchange parameters deduced from the high temperature susceptibility implies on its own the existence of a yet unknown phenomena which promotes the FM hard axis ordering at low temperature. Thus this analysis provides further support for the main conclusion

of our paper.

In this context it is interesting to note that the same contradiction was also observed in the case of a Kondo lattice which orders antiferromagnetically along the hard CEF axis:  $\text{CeRu}_2\text{Al}_{10}$ . This orthorhombic system belongs to a whole family of compounds which has encountered strong interest because of a number of unusual properties [58]. In  $\text{CeRu}_2\text{Al}_{10}$  a number of properties and studies conclusively indicate that the CEF ground state doublet presents a large moment  $m_a \approx 1.44 \mu_B$  along the  $a$  direction, a much weaker moment  $m_c \approx 0.38 \mu_B$  along the  $c$  direction, and an even weaker moment along the  $b$  direction,  $m_b = 0.19 \mu_B$  [56]. However it has been unambiguously shown that the AFM ordered moment is predominantly along the hard  $c$  direction [57]. The magnetic excitations in the ordered states have been determined using INS [55], and the analysis of these INS data using a similar approach as in [37] resulted in a huge anisotropy of exchange interactions, those for the  $c$ -component of the moments being a factor of 50 larger than those for the  $a$  or the  $b$ -component [55]. However comparing the CEF and the measured susceptibilities at high temperature also indicate the anisotropy of the mean field exchange parameters at high temperatures to be at least one order of magnitude smaller, not larger than a factor of 4, with  $\lambda_a < \lambda_c < \lambda_b$ . Thus, as in  $\text{CeAgSb}_2$ , the exchange parameters and their anisotropy required by the hard-axis ordering in  $\text{CeRu}_2\text{Al}_{10}$  within a mean field approach are incompatible with the exchange parameters and their anisotropy deduced from the high temperature susceptibilities. In this case the authors of [55] themselves concluded that this type of analysis results in an “unrealistically large  $J_c$  value”. These observation in the AFM system  $\text{CeRu}_2\text{Al}_{10}$  evidence that the problem we addressed and discussed for FM systems is also of relevance for AFM systems, and thus seems to be more general.

- 
- [34] K. Myers *et al.*, J. Magn. Magn. Mater. **205**, 27 (1999).
  - [37] S. Araki *et al.*, Phys. Rev. B **68**, 024408 (2003).
  - [39] E. Jobiliong, J. S. Brooks, E. S. Choi, H. Lee, and Z. Fisk, Phys. Rev. B **72**, 104428 (2005).
  - [55] J. Robert *et al.*, Phys. Rev. Lett. **109**, 267208 (2012).
  - [56] F. Strigari *et al.*, Phys. Rev. B **86**, 081105 (2012).
  - [57] P. Dean, Y. Muro, T. Takabatake, and P. D. Hatton, J. Phys. Soc. Jpn. **87**, 013706 (2018).
  - [58] D. T. Adroja *et al.*, Phys. Scr. **88**, 068505 (2013).
  - [S1] P. Boutron, Phys. Rev. B **7**, 3226 (1973).
  - [S2] M. A. Adroja, S. L. Bud'ko, and P. C. Canfield, J. Magn. Magn. Mater. **270**, 51 (2004).
